# Supplementary material for: In-Context Learning for Robots: Methods and Applications
Source: arXiv:2609.36012 source file (2026-09-28)
Supplement: Supplementary file 1 [file 15-notation-appendix.tex]

\FloatBarrier
\suppressfloats[t]
% Keep the heading and first semantic group together; allow continuation by group.
\Needspace*{18\baselineskip}
\section{Notation}
\label{app:notation}
\setcounter{table}{0}
\renewcommand{\thetable}{\thesection\arabic{table}}
\renewcommand{\theHtable}{\thesection\arabic{table}}

Neural parameters are separated from changing context, internal state, and retained artifacts.

\begingroup
\surveytable
\renewcommand{\arraystretch}{1.26}
\setlength{\LTleft}{\fill}\setlength{\LTright}{\fill}
\setlength{\LTpre}{8pt}\setlength{\LTpost}{6pt}
\begin{longtable}{@{}>{\raggedright\arraybackslash}p{.26\linewidth}>{\raggedright\arraybackslash}p{\dimexpr.74\linewidth-2\tabcolsep\relax}@{}}
\caption{Shared notation by role. Superscripts $\mathrm{s}$ and $\mathrm{q}$ denote support and query; other \mbox{symbols are defined locally.}}\label{tab:notation}\label{discuss:tab:notation}\\
\toprule
\textbf{Symbol} & \textbf{Meaning}\\
\midrule
\endfirsthead
\caption[]{Shared notation (continued).}\\
\toprule
\textbf{Symbol} & \textbf{Meaning}\\
\midrule
\endhead
\bottomrule
\endfoot

\rowcolor{panel}[0pt][0pt]\multicolumn{2}{@{}l@{}}{\strut\textbf{Decisions, evidence, and retained state}}\\*
$t$, $n$ & Robot decision step; complete-attempt index.\\*
$i$, $j$, $\ell$, $b$ & Demonstration element; memory record; skill; motion segment.\\*
$o_t$, $a_t$, $h_t$ & Observation; executed command; observation--action history.\\*
$A_t$, $\widehat a_{t+\omega\mid t}$, $H$ & Proposed action block; action at offset $\omega$; block horizon.\\*
$D^{\mathrm s}$, $L$, $d_i^{\mathrm s}$ & Support demonstration; demonstration length; demonstration element.\\*
$C_t$, $C_t^{\mathrm{task}}$, $r_t$ & Policy context; supplied task evidence; interpreted representation.\\*
$m_t$, $M_t$, $R_t$ & Recurrent state; external archive; retrieved records.\\*
$x_t$, $\xi_j$, $J_t$, $N_t$ & Executed transition; archive record; selected indices; archive size.\\*
$B_n$, $\widetilde B_{n+1}$ & Retained external artifacts; proposed revision.\\*
$\mathcal T_n$, $\chi_n$ & Attempt trace with feedback; revision-acceptance indicator.\\
\rowcolor{panel}[0pt][0pt]\multicolumn{2}{@{}l@{}}{\strut\textbf{Method families and their components}}\\*
$\theta$, $\theta_0$ & Neural parameter collection; deployment initialization.\\
$\bar\theta$, $\phi_t$ & Frozen backbone; adaptive neural subset in TTT.\\
$\pi_\theta$ & Conditional distribution of the next action block.\\
$E_\theta^{\mathrm c}$, $E_\theta^{\mathrm m}$ & Context interpreter; demonstration motion-descriptor extractor.\\
$q_\theta^{\mathrm a}$, $q_\theta^{\mathrm v}$ & Action generators conditioned on a representation or a predicted future.\\
$v^+$, $p_\theta^{\mathrm v}$, $p_\theta^{\mathrm d}$ & Anticipated future; context-conditioned prediction; action-conditioned dynamics.\\
$g$, $f_\theta$, $p_\theta^{\mathrm g}$ & Execution specification; deterministic or stochastic specification generator.\\
$\kappa$, $k_\theta$, $\kappa_{B_n}$ & Deterministic, stochastic, and artifact-dependent executors.\\
$z_\ell$, $N_g$, $\ell_t$ & Skill specification; number of skills; active skill index.\\
$\zeta_i$, $\mathcal B$ & Motion descriptor; robot kinematics and control description.\\
\rowcolor{panel}[0pt][0pt]\multicolumn{2}{@{}l@{}}{\strut\textbf{Training and evaluation}}\\*
$\psi$, $\tau^{\mathrm q}$, $P_{\mathrm{pair}}$ & Task specification; query trajectory; support--query pair distribution.\\
$I^{\mathrm q}$, $\ell_\theta$, $\mathcal L$ & Supervised query positions; per-target action loss; expected training loss.\\
$S_n$, $\Delta_n^{\mathrm{reuse}}$ & Success/adherence rate; gain from retained evidence at attempt $n$.\\
\end{longtable}
\par\phantomsection\label{floatend:tab:notation}
\endgroup
